# Supplementary material for: Raman scattering from current-stabilized nonequilibrium phases in Ca$_2$RuO$_4$
Source: arXiv:1907.07905 ancillary file (2019-07-22)
Supplement: Supplementary file 1 [file supp.pdf]

# Supplementary Information for “Raman scattering from current-stabilized nonequilibrium phases in $\text{Ca}_2\text{RuO}_4$ ”

K. Fürsich,<sup>1</sup> J. Bertinshaw,<sup>1</sup> P. Butler,<sup>1</sup> M. Krautloher,<sup>1</sup> M. Minola,<sup>1,\*</sup> and B. Keimer<sup>1,†</sup>

<sup>1</sup>*Max-Planck-Institut für Festkörperforschung, Heisenbergstrasse 1, 70569 Stuttgart, Germany*

(Dated: July 17, 2019)

## I. TEMPERATURE-DRIVEN INSULATOR-TO-METAL TRANSITION STUDIED WITH RAMAN LIGHT SCATTERING — THE $L$ -PHASE

We also investigated the temperature-induced insulator-to-metal transition in  $\text{Ca}_2\text{RuO}_4$  to obtain the equilibrium  $S$ - and  $L$ -phases<sup>1–4</sup> in Fig. S1. The Raman experiments were performed on the very same crystal from the main text mounted in a Linkam cryostat to facilitate measurements up to 450 K. Note that for the specific set-up used here, we give an error in temperature of  $\pm 10$  K.

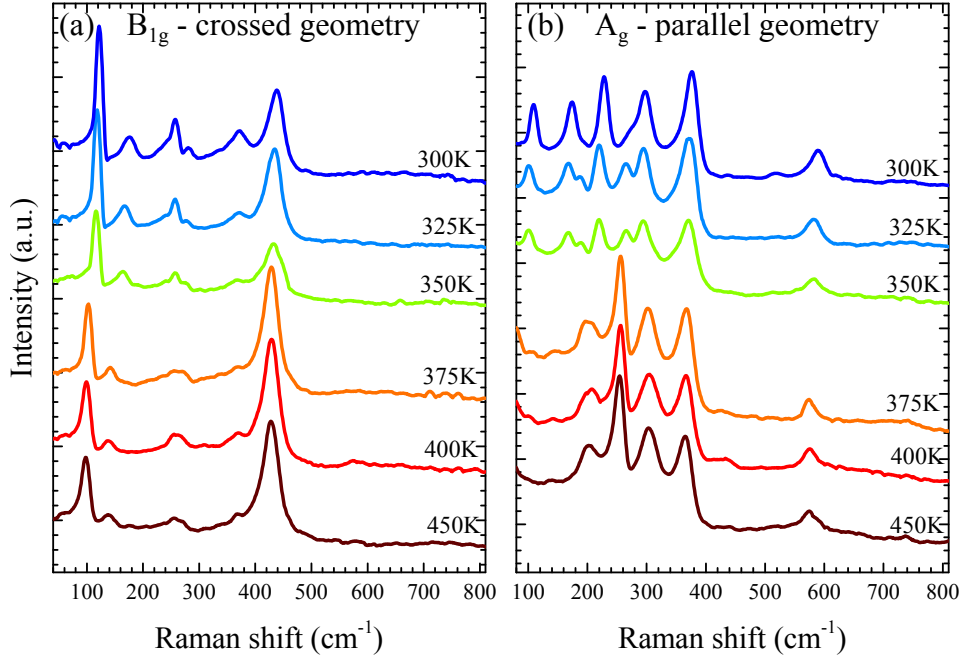

FIG. S1. Temperature-induced IMT in  $\text{Ca}_2\text{RuO}_4$ . (a) and (b) Temperature-dependent Raman spectra in  $B_{1g}$  and  $A_g$  geometry, respectively.

## II. DETAILS ON RAMAN CRYOSTAT, SAMPLE MOUNTING AND COOLING PROCEDURE

As the cooling procedure turns out to be crucial to observe the current-stabilized nonequilibrium phases in  $\text{Ca}_2\text{RuO}_4$ , we give details about the sample mounting and cooling system used in our experiment. Fig. S2 (a) shows an overview of the commercially available KONTE cryostat from CryoVac. We highlighted the path of the He flow as well as the cables which were installed to apply a DC current to the sample. In panel (b) of Fig. S2, we schematically illustrate the sample mounting using GE varnish, which electrically isolates the sample from the metallic sample holder while at the same time providing good thermal contact to the latter. The sample holder essentially acts as a cold finger. The sample is contacted to standard Cu wires with conductive silver paint. A detailed photograph of the sample environment is shown in panel (c).

The experiments were carried out in the voltage-controlled mode. We used silver epoxy to contact the samples in a two-probe circuit and a Keithley 2400 Source Measure Unit for sampling and control. The laser spot size of our micro-Raman setup is  $1.4\,\mu\text{m}$ . Raman scattering is a bulk sensitive probe, where the probing depth is given by

the penetration depth of the laser beam. The penetration depth for a red laser in transition metal oxides such as  $\text{Ca}_2\text{RuO}_4$  is around  $3\mu\text{m}$ .

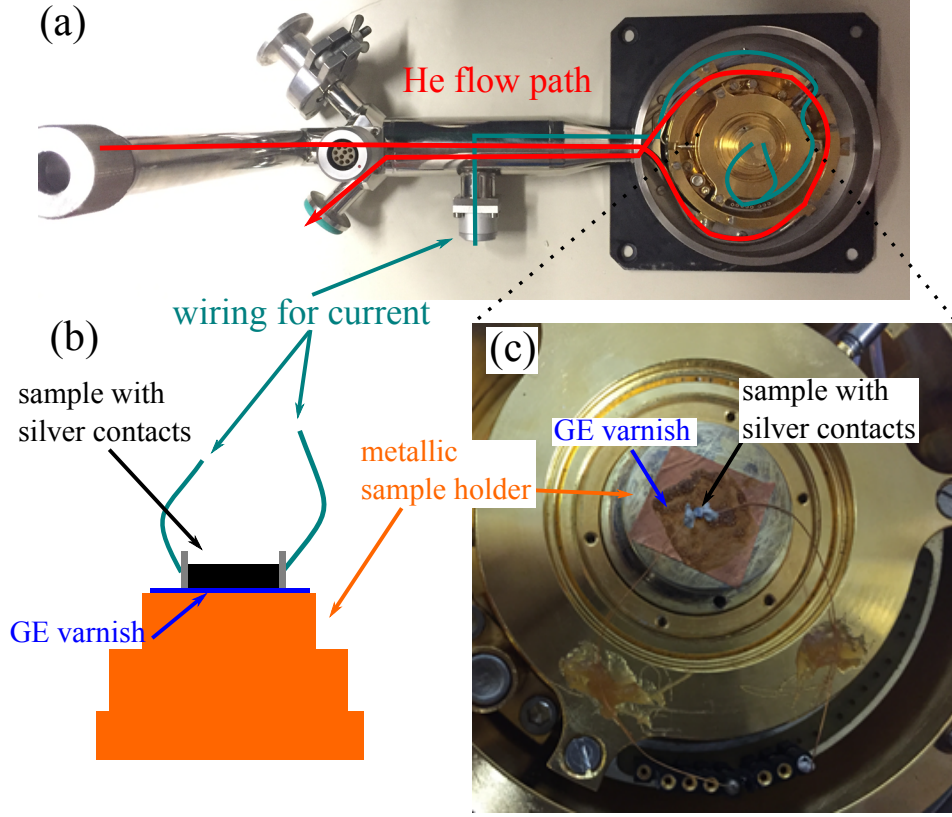

FIG. S2. (a) Photo of the Raman cryostat, where the He flow path is marked in red and the wiring to apply current in green. (b) Schematics of the sample mounting on the metallic sample holder. (c) Detailed photograph of the sample mounted in the cryostat.

### III. STOKES/ANTI-STOKES ANALYSIS

Here, we exemplify the Stokes/anti-Stokes analysis for the 93mA data at 250K. The spectrum is fitted by a superposition of Voigt profiles with an additional linear background (see Fig. S3). This procedure is standard in the analysis of Raman spectra as the Voigt profile accounts for both experimental resolution and intrinsic lifetime broadening<sup>5,6</sup>. To evaluate the temperature following equation 1 from the main text, we need to compare the intensities of Stokes and anti-Stokes profiles for a specific phonon<sup>7,8</sup>. This is illustrated in Fig. S3, where the corresponding Stokes and anti-Stokes phonons are marked with the same color. The temperatures given in the table of the main text come from the average of the temperatures determined for all visible phonons of one spectrum. We emphasize that one can determine the actual *in-situ* temperature  $T$  at the laser spot. This accounts for possible effects of laser heating<sup>9</sup> and, in the present work, of current-induced Joule heating.

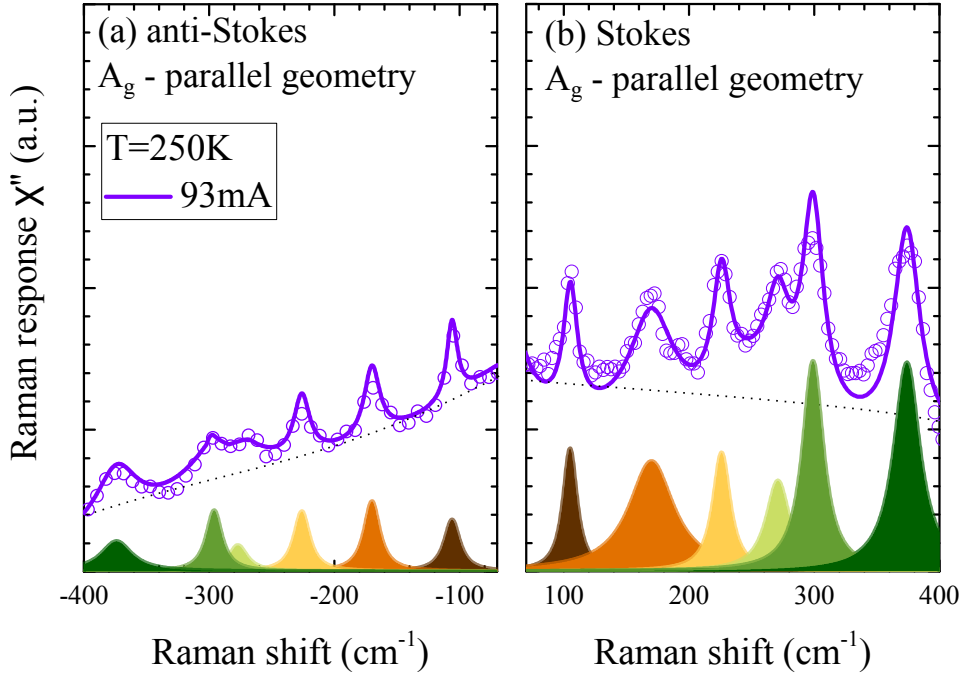

FIG. S3. Raman spectra in the parallel  $A_g$  channel for (a) anti-Stokes and (b) Stokes regions, respectively. Each experimental spectrum is fitted by a superposition of several Voigt profiles and a linear background. The Voigt peaks are shown at the bottom. The dotted line shows the linear background. Corresponding phonons of the Stokes and anti-Stokes sides of the spectra are marked with the same color.

#### IV. TEMPERATURE EVALUATION AT $T = 10$ K WITH AND WITHOUT APPLIED CURRENT

Hereafter, we discuss our Raman thermometry scheme which allows us to exclude heating effects at  $T = 10$  K. The anti-Stokes side of the spectrum at  $T = 10$  K is essentially featureless (see Fig. S4), which is expected from the Bose statistics<sup>7,8</sup>. This observation holds for both measurements with and without current. Therefore, we cannot apply the methodology used to extract the temperature at  $T = 250$  K. However, as we have shown in the first part of the main text and illustrated in detail in the previous section, heating can be neglected at much higher currents with lower cooling power (due to the higher temperature) of the sample. Together with the absence of the anti-Stokes features with (and without) applied current, this demonstrates the absence of any substantial heating in the low-current regime at  $T = 10$  K.

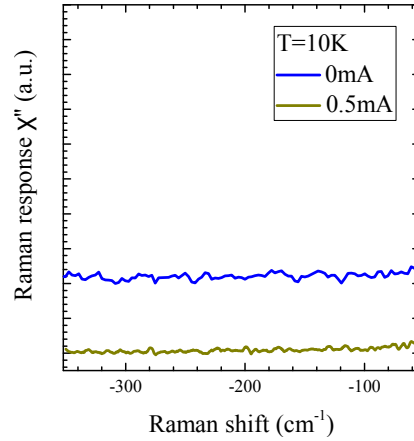

FIG. S4. Anti-Stokes part in parallel  $A_g$ -geometry at 10 K with and without applied current. For the Stokes part of the spectrum, see Fig. 4(b) of the main text. The data for 0 mA is offset for clarity.

## V. $R(V)$ CURVES WITH AND WITHOUT COOLING

For a more comprehensive overview of transport data, we give  $R(V)$  curves in addition to the  $I(V)$  data of the main text [Figs. 1(a) and 2(a)]. Both panels of Fig. S5 show two different regimes with higher resistance  $R_{\text{ins}}$  and lower one  $R_{\text{m}}$ , corresponding to insulating and metallic regimes, thereby confirming the insulator-to-metal transition<sup>10</sup>. We point out that our data was taken in the voltage-controlled mode, which is why we use  $U(V)$  as the horizontal axes of the transport plots.

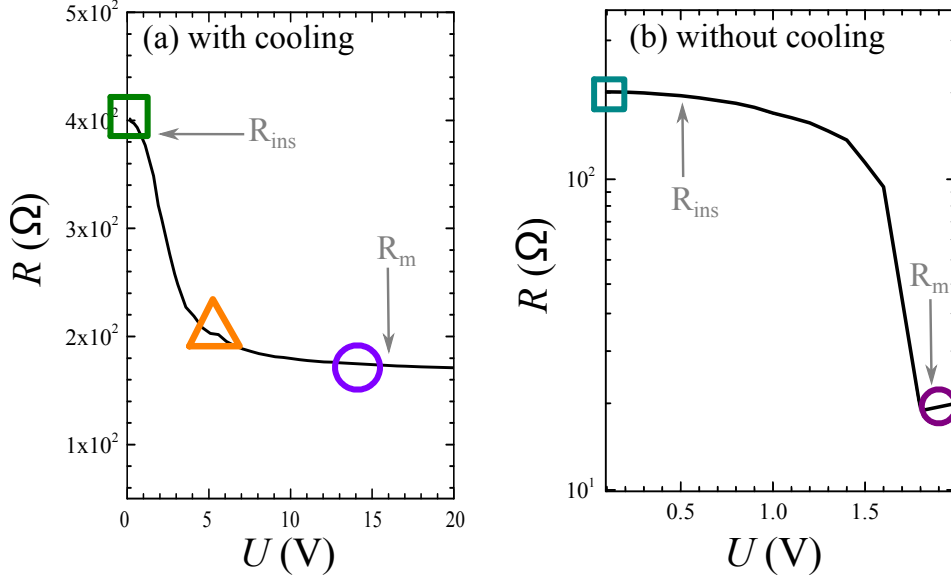

FIG. S5.  $R(V)$  curves (a) with cooling and (b) without cooling. In (a) the arrows illustrate two regions with different resistance, i.e. insulating ( $R_{\text{ins}}$ ) and metallic ( $R_{\text{m}}$ ) state.

## VI. COMMENTS ABOUT SAMPLE HISTORY AND REPRODUCIBILITY

The history of a specific sample can affect the physical properties determined in systems that show a first-order structural phase transition. Therefore it is crucial to consider the electric or thermal cycles when discussing results in materials such as  $\text{Ca}_2\text{RuO}_4$ . As far as the low current regime is concerned, we noticed neither damage to the samples nor changes in the samples' properties. Even after a thermal cycle (300K-10K-300K) with or without applied current the resistance under ambient conditions did not change. The findings in the high current regime were reproduced for samples which had experienced a thermal cycle (300K-10K-300K) and for those that did not. For both scenarios, we observed the same key spectral features in the  $L^*$  phase. Detectable sample damage only occurred for samples driven into the  $L$ -phase, where small cracks were observed that led to a loss of conductivity across the samples when  $\text{Ca}_2\text{RuO}_4$  transitioned from the  $L^*$ - to the  $S$ -phase.

All major findings were reproduced multiple times with different samples. We can thus safely conclude that the current-stabilized phases are distinct from the equilibrium ones and that the long-range magnetic order is suppressed. Additionally, we made sure that any conclusion on heating- and current-induced effects is independent from any sample-specific history.

---

\* [M.Minola@fkf.mpg.de](mailto:M.Minola@fkf.mpg.de)

† [B.Keimer@fkf.mpg.de](mailto:B.Keimer@fkf.mpg.de)

<sup>1</sup> H. Rho, S. L. Cooper, S. Nakatsuji, H. Fukazawa, and Y. Maeno, *Phys. Rev. B* **68**, 100404 (2003).

<sup>2</sup> J. Jung, *Solid State Commun.* **133**, 103 (2005).

<sup>3</sup> H. Rho, S. L. Cooper, S. Nakatsuji, H. Fukazawa, and Y. Maeno, *Phys. Rev. B* **71**, 245121 (2005).

<sup>4</sup> S.-M. Souliou, J. Chaloupka, G. Khaliullin, G. Ryu, A. Jain, B. J. Kim, M. Le Tacon, and B. Keimer, *Phys. Rev. Lett.* **119**, 067201 (2017).

- <sup>5</sup> H. Gretarsson, N. H. Sung, M. Höppner, B. J. Kim, B. Keimer, and M. Le Tacon, [Phys. Rev. Lett. \*\*116\*\*, 136401 \(2016\)](#).
- <sup>6</sup> C. Ulrich, G. Khaliullin, M. Guennou, H. Roth, T. Lorenz, and B. Keimer, [Phys. Rev. Lett. \*\*115\*\*, 156403 \(2015\)](#).
- <sup>7</sup> M. Cardona and G. Güntherodt, [\*Light Scattering in Solids II: Basic Concepts and Instrumentation\*](#), Vol. 50 (Springer, 1982).
- <sup>8</sup> W. Hayes and R. Loudon, *Scattering of Light by Crystals* (Dover Publications, Inc., Mineola, NY, 2004).
- <sup>9</sup> We kept our laser power well below 1 mW to avoid laser heating.
- <sup>10</sup> M. Braden, G. André, S. Nakatsuji, and Y. Maeno, [Phys. Rev. B \*\*58\*\*, 847 \(1998\)](#).
